# Supplementary material for: Hole Transport in Exfoliated Monolayer MoS$_2$
Source: arXiv:1804.09218 ancillary file (2018-04-24)
Supplement: Supplementary file 1 [file Supporting_information_MoS2_hole_transport_Ponomarev.pdf]

# Supporting information for the manuscript

# “Hole Transport in Exfoliated Monolayer $MoS_2$”

*By Evgeniy Ponomarev, Árpád Pásztor, Adrien Waelchli, Alessandro Scarfato, Nicolas Ubrig, Christoph Renner, and Alberto F. Morpurgo*

## 1. FET transfer curves with Pt and Au contacts

In the main text we mention that the anomalous current suppression in the hole accumulation region occurs irrespective of the material used to realize the source and drain contacts. This is illustrated by Figure S1, which shows transfer characteristics in devices fabricated with Au and Pt contacts. In both cases we observe an abrupt drop of conductivity $\sigma_\square$ at the onset of hole conduction. The small relative shift in gate voltage between the curves can be fully accounted for by the difference in the work function of the Au and Pt contacts.

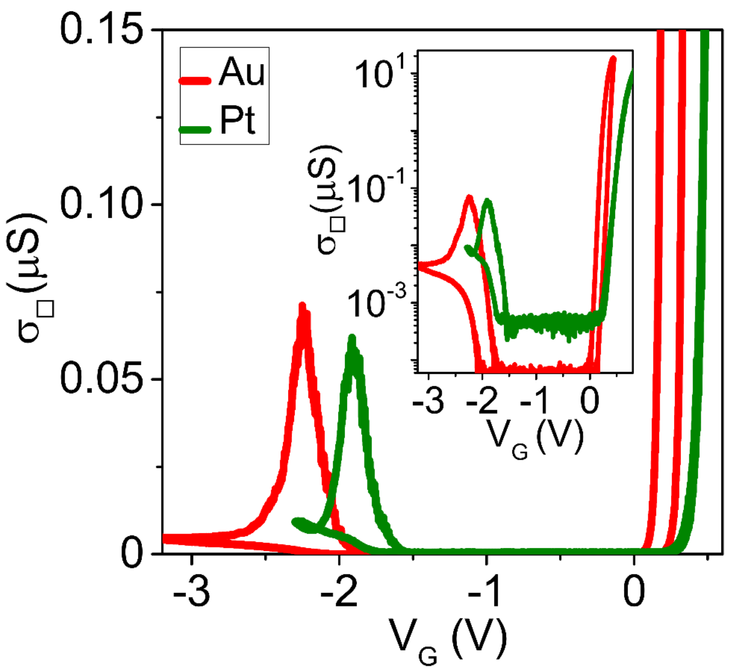


**Figure S1.** Comparison of FET transfer characteristics measured on monolayer $MoS_2$ devices with different contact materials (red curve – Au contacts, green curve – Pt contacts). (Inset) Semilogarithmic plots of the data shown in the main panel.

## 2. Photoluminescence map

In figure S2 we show a map of normalized photoluminescence intensity acquired as a function of gate voltage and wavelength together with the corresponding FET transfer curve (black line). Irrespective of the applied gate voltage the position of the peak which arises from A-exciton recombination in monolayer $MoS_2$ (at about 670 nm) remains unchanged. Upon charge accumulation in the conduction band and at the onset of the valence band photoluminescence spectra broadens, possibly due to a decrease of exciton lifetime caused by screening of the carriers, or because of the simultaneous presence of excitons and trions. Note that the FET transfer curve measured at the same time is shifted towards more negative $V_G$ values as compared to the one shown in figure 1b of the main text because of bias stress caused by the extended measurements performed on this device.

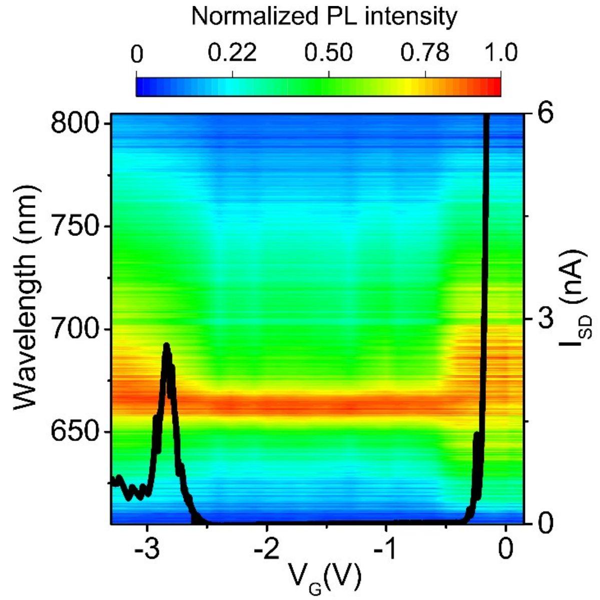


**Figure S2.** Map of normalized photoluminescence intensity as a function of gate voltage and wavelength. The black curve is the FET transfer characteristic (see legend on the right axis, $V_{SD}$ = 20mV).

### 3. FET transfer curve at reduced temperature

In the main text we have explained that hole transport in monolayer $MoS_2$ is anomalous due to strong trapping of holes by defect states having energy near the top of the valence band. It is therefore expected that upon lowering sample temperature hole conduction should be strongly suppressed. This is indeed what happens, as illustrated in figure S3, where transfer curves measured at T = 270 K and 300 K are shown. In the anomalous transport region the onset of hole conduction seen at 300K is no longer observed at 270K and the source-drain current drops below the noise floor of the measurement. Note that on the electron side the two curves look almost identical compatibly with the fact that electron transport is mediated by carriers in band states (and not by trapped carriers).

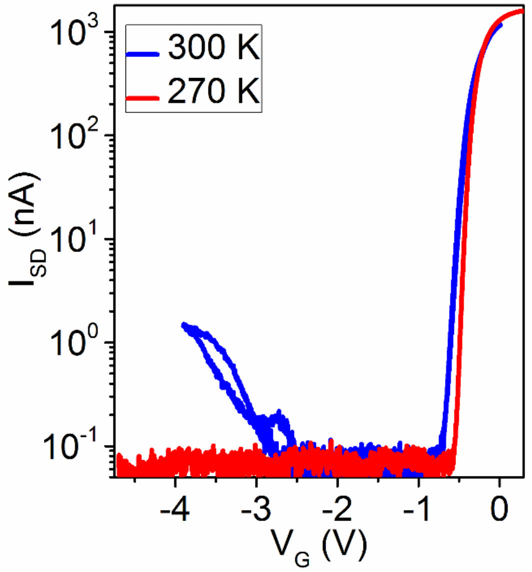


**Figure S3.** Transfer curves of monolayer $MoS_2$ FET measured at T=300 K (blue curve) and at T=270K (red curve).
